# Supplementary material for: Memories of amplitude and direction coexist and compete in non-Brownian suspensions
Source: arXiv:2510.11825 ancillary file (2026-05-01)
Supplement: Supplementary file 1 [file SAMIRONB_Supplementary_Material.pdf]

# Supplementary Material

## MIRROR SYMMETRY

We verified that all our results were invariant under the transformation $\gamma \to -\gamma$ by performing a mirror counterpart to each experiment. Figure S1 shows example protocols that are mirror images of those shown in Fig. 2(a & b) of the main text. The resulting viscosity signals in Fig. S1(c) match the original readouts of Fig. 2(c) of the main text. We found excellent agreement in all of the mirror cases, which is expected since there is no inherent preference for a direction in our instrument or sample.

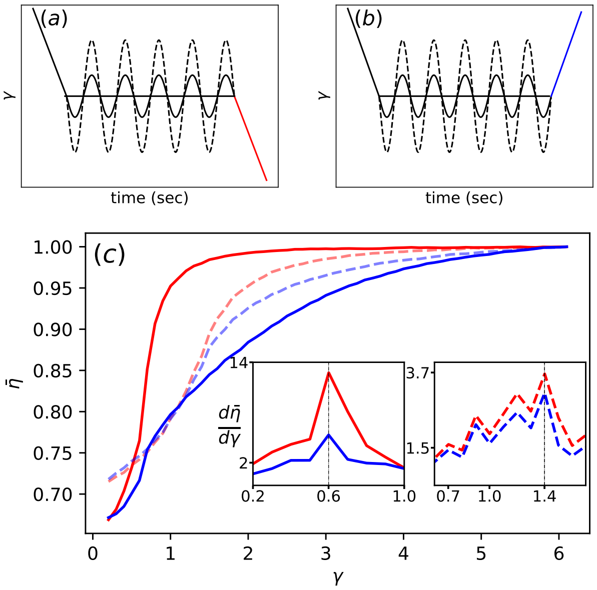


FIG. S1. **Protocols testing mirror symmetry:** Protocols in (a) and (b) are mirror inversions of the protocols in Fig. 2(a & b) of the main text. The response in (c) matches the response in Fig. 2(c) of the main text, as expected.

## VISCOUS HEATING

Despite the rheometer maintaining the outer cylinder's constant temperature, the non-normalized fluid viscosity gradually decreases over many closely spaced experiments, which we attribute to viscous heating within the sample. As shown in Fig. S2(a), the apparent steady-state viscosity at large strain should be independent of history, but instead decreases as we perform successive trials at increasing $\gamma_T$. We verified the role of viscous heating by performing a subset of experiments at a tenth of the usual strain rate, 0.01 s$^{-1}$, to reduce total dissipation and to allow better cooling of the entire sample through heat transfer at the outer boundary. Results in Fig. S2(b) agree qualitatively with our other memory experiments, but are much noisier due to the smaller torque. The spread of final viscosities is much smaller, consistent with reduced viscous heating. The effective viscosity $\eta$ of an un-jammed suspension is expected to scale linearly with the liquid viscosity $\eta_l$, and the ratio $\eta/\eta_l$ should be history-independent at large strain, which we take to be $\gamma = 6$. Therefore all our other plots and calculations use the normalized viscosity $\bar{\eta}$, which removes heating effects by dividing each raw viscosity curve by its value at $\gamma = 6$.

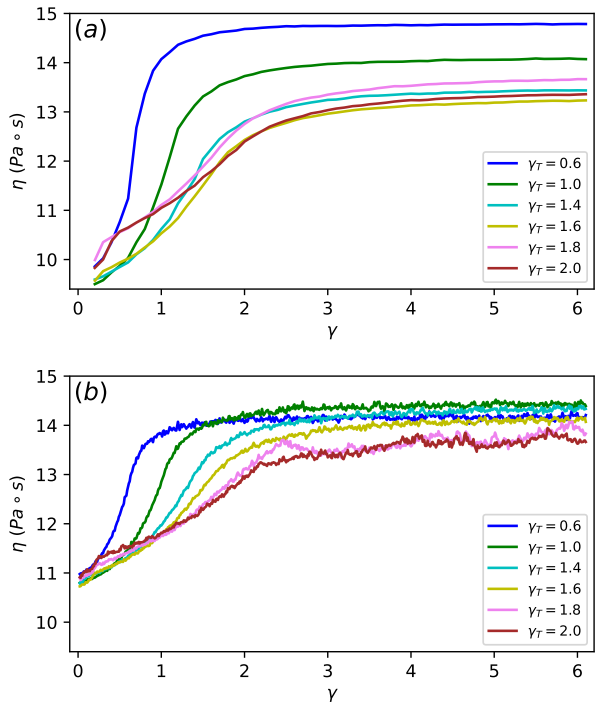


FIG. S2. **Effects of viscous heating. (a)** Readout curves from a consecutive series of trials at varying $\gamma_T$, with a maximum strain rate of 0.1 s$^{-1}$, show different steady-state viscosities near $\gamma = 6$, implying that fluid viscosity decreases by $\sim 15\%$. **(b)** Data from the same protocols, performed 10 times slower (maximum strain rate 0.01 s$^{-1}$) to reduce viscous heating. The viscosities near $\gamma = 6$ are now more closely spaced, varying by only $\sim$5%.

## PREPARING VISCOSITY DATA FOR $\delta$

To compute $\delta$ from readout data, we must first ensure that we compare steady-shear viscosity measurements

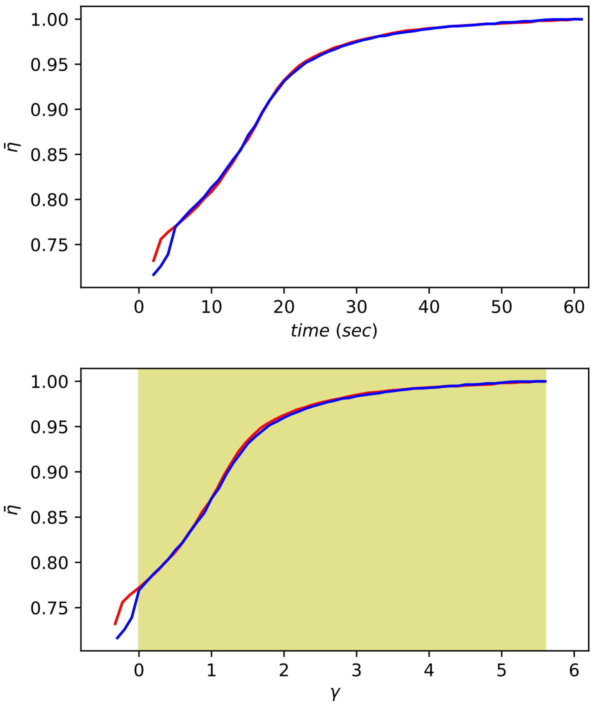


FIG. S3. **Strain during readout. Top panel:** Normalized viscosity during readout. The rheometer samples viscosity every 0.1 s. Data correspond to the protocols in Fig. 2 (a & b) of the main text, at $\gamma_T = 1.8$. **Bottom panel:** The same curves replotted in strain, and shifted so that $\gamma = 0$ corresponds to the midpoint of oscillatory training. In this shifted strain, we use only $\gamma \geq 0$ (yellow shaded region) when computing $\delta$.

that were taken as close as possible in $|\gamma|$, with respect to the midpoint of oscillatory training $\gamma = 0$. Our oscillatory training protocols end slightly before they reach $\gamma = 0$, causing the readout to start at a small nonzero strain that depends on the shear direction and that is proportional to $\gamma_T$. An example symmetric pair of readouts with $\gamma_T = 1.8$ is plotted in Fig. S3(a), as a function of time during the rheometer's readout test. The rheometer records samples at a fixed rate of 1 Hz. In Fig. S3(b) we replot the data against strain, using the nominal strain rate of 0.1 $\mathrm{s}^{-1}$. We account for the strain offsets by shifting each curve by the nearest integer number of samples (i.e. increments of 0.1 in strain). The limited precision simplifies computing $\delta$ by keeping samples aligned.

We also observe an initial transient in the data, possibly due to deviations from constant strain rate as the rheometer test begins. We ignore this transient by only considering data for $\gamma \geq 0$.

Finally, we note that the net effect of correcting for these details of rheometer operation is relatively small, reducing $\delta$ by $\mathcal{O}(10^{-3})$ to $\mathcal{O}(10^{-2})$, even at large $\gamma_T$. The corrections do not change our qualitative results nor the apparent values of $\gamma_m^*$ and $\gamma_b^*$.

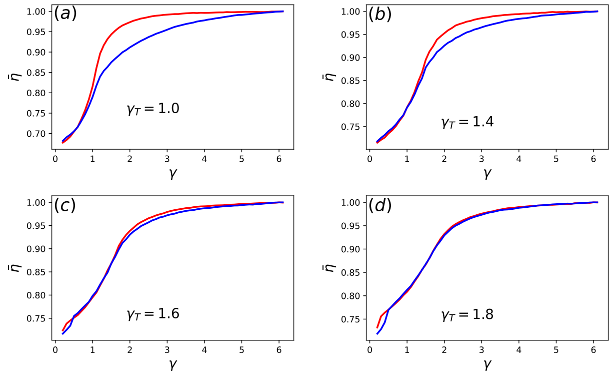


FIG. S4. **Fore-aft asymmetry vanishes with increasing training amplitude.** The four figures (a, b, c, and d) illustrate the suspension's response to the protocol depicted in Fig. 2(a & b) of the main text. Readout matches the direction of preparation (Red) and is in the opposite direction (Blue). It's evident that the $\delta$ value decreases as we transition from $\gamma_T = 1.0$ to 1.8. Notably, the curves essentially overlap for $\gamma_T \geq 1.8$. This suggests that the suspension exhibits symmetry in both clockwise and counterclockwise steady shear about $\gamma = 0$. In essence, this indicates the disappearance of any fore-aft asymmetry.

## VISCOSITY CURVES USED FOR MEASURING ASYMMETRY

Figure S4 shows the normalized viscosity curves during readout, from the "match" protocols in Fig. 2(a & b) of the main text at four values of the training amplitude $\gamma_T$. The strain shift in Fig. S3 has not yet been applied. As $\gamma_T$ increases, the curves grow more similar, and the area $\delta$ between them decreases, as plotted with magenta points in Fig. 3 of the main text. The curves nearly coincide when $\gamma_T \geq 1.8$. The mismatch around $\gamma < 0.5$ in panels (c & d) are attributed to the initial transient discussed in the previous section.
